# Supplementary material for: Are Your Reviewers Being Treated Equally? Discovering Subgroup Structures to Improve Fairness in Spam Detection
Source: arXiv:2204.11164 source file (2023-05-05)
Supplement: Supplementary file 1 [file appendices.tex]

\section{Appendix}
\begin{table*}
    \centering
    \small 
    \caption{NDCG values for the outputs of spam detectors on three Yelp datasets.
    Shown are the average results over all different splits.
    ``\textbf{\textcolor{red}{*}}'' denotes our method. \textcolor{red}{Add that the lower the metric the better.}}
    \resizebox{\textwidth}{!}{
    \begin{tabular}{c|c|c c c | c c c |c c c}
    \toprule
        \textbf{Detector} & \textbf{NDCG(\%)} & \multicolumn{3}{c|}{\textbf{Chi}} & \multicolumn{3}{c|}{\textbf{NYC}} & \multicolumn{3}{c}{\textbf{Zip}} \\  
         \cline{1-11}
        \multirow{3}*{\textbf{FairGNN}~\cite{dai2021say}} & $\mathcal{V}^R$ & \multicolumn{3}{c|}{86.2\tiny{$\pm $0.1}} & \multicolumn{3}{c|}{85.9\tiny{$\pm $0.0}}  & \multicolumn{3}{c}{89.6\tiny{$\pm $0.5}} \\
        ~ & $\mathcal{V}^R_1$ & \multicolumn{3}{c|}{86.2\tiny{$\pm $0.1}} & \multicolumn{3}{c|}{86.0\tiny{$\pm $0.0}}  & \multicolumn{3}{c}{89.6\tiny{$\pm $0.4}} \\
        \rowcolor{gray!20}
         \cellcolor{white} ~ & $\Delta_{\text{NDCG}}$ & \multicolumn{3}{c|}{53.7\tiny{$\pm $2.1}} & \multicolumn{3}{c|}{20.7\tiny{$\pm $1.1}} & \multicolumn{3}{c}{36.4\tiny{$\pm $4.6}} \\
        \cline{1-11}
         \multirow{3}*{\textbf{EDITS}~\cite{dong2022edits}} & $\mathcal{V}^R$ & \multicolumn{3}{c|}{84.3\tiny{$\pm $0.3}} & \multicolumn{3}{c|}{84.9\tiny{$\pm $0.1}} & \multicolumn{3}{c}{89.2\tiny{$\pm $0.0}} \\
          ~ & $\mathcal{V}^R_1$ & \multicolumn{3}{c|}{84.3\tiny{$\pm $0.3}} & \multicolumn{3}{c|}{85.1\tiny{$\pm $0.1}} & \multicolumn{3}{c}{89.3\tiny{$\pm $0.0}}\\
        \rowcolor{gray!20} 
         \cellcolor{white} ~ & $\Delta_{\text{NDCG}}$ & \multicolumn{3}{c|}{50.9\tiny{$\pm $2.3}} & \multicolumn{3}{c|}{32.7\tiny{$\pm $1.5}} & \multicolumn{3}{c}{39.4\tiny{$\pm $10.6}} \\
        \cline{1-11}
        \midrule
          \multirow{2}*{\textbf{Detector}}&  \multirow{2}*{\textbf{NDCG(\%)}}  & \multicolumn{3}{c|}{\textbf{GNN}$(g_{\boldsymbol{\theta}})$} & \multicolumn{3}{c|}{\textbf{GNN}$(g_{\boldsymbol{\theta}})$} & \multicolumn{3}{c}{\textbf{GNN}$(g_{\boldsymbol{\theta}})$}\\
         &   ~&  \textbf{w/o} & \textbf{Pre-trained} &  \textbf{Joint\textcolor{red}{*}}& \textbf{w/o} & \textbf{Pre-trained} &  \textbf{Joint\textcolor{red}{*}} & \textbf{w/o} & \textbf{Pre-trained} &  \textbf{Joint\textcolor{red}{*}}\\
         \cline{1-11}
     \multirow{3}*{\textbf{GNN}} &  $\mathcal{V}^R$ & 84.5\tiny{$\pm$0.9}  & 83.2\tiny{$\pm $1.5} & 83.3\tiny{$\pm $2.2}  & 85.2\tiny{$\pm $0.8} & 85.1\tiny{$\pm$0.8} &  85.2\tiny{$\pm$0.5} & 88.4\tiny{$\pm$1.4} & 87.6\tiny{$\pm$1.5} & 88.6\tiny{$\pm$1.0}\\    
        ~ & $\mathcal{V}^R_1$ & 84.7\tiny{$\pm $0.9} & 83.5\tiny{$\pm $1.3} & 83.6\tiny{$\pm $2.1} & 85.1\tiny{$\pm$ 0.8} & 85.3\tiny{$\pm$0.8} & 85.2\tiny{$\pm$0.5} & 88.4\tiny{$\pm$1.4} & 87.6\tiny{$\pm$1.5} & 88.6\tiny{$\pm$1.0}\\
      \rowcolor{gray!20} 
     \cellcolor{white} ~ & $\Delta_{\text{NDCG}}$ & 51.2\tiny{$\pm $2.1} & 51.0\tiny{$\pm $3.0} & \textbf{50.7}\tiny{$\pm $3.5}  & 21.9\tiny{$\pm$7.0} & 21.8\tiny{$\pm$7.8} & \textbf{21.3}\tiny{$\pm$8.9} &  36.3\tiny{$\pm$10.4} & \textbf{34.3}\tiny{$\pm$10.8} &  34.8\tiny{$\pm$11.1}\\     % delta ndcg
     \cline{1-11}
         \multirow{3}*{\textbf{GNN-}$\mathbf{S_{1}^{\textbf{Tr}}}$\textbf{\textcolor{red}{*}}} &  $\mathcal{V}^R$ & 85.6\tiny{$\pm $0.7} & 85.8\tiny{$\pm $0.5} & 85.6\tiny{$\pm $0.8}  & 85.8\tiny{$\pm$0.1} & 85.9\tiny{$\pm$0.0} &  85.9\tiny{$\pm$0.0} &  89.7\tiny{$\pm$0.2} & 89.7\tiny{$\pm$0.1} & 89.6\tiny{$\pm$0.1}\\
      ~  & $\mathcal{V}^R_1$ & 85.6\tiny{$\pm $0.7} & 85.8\tiny{$\pm $0.5} & 85.7\tiny{$\pm $0.8}  & 85.9\tiny{$\pm$0.0} & 86.0\tiny{$\pm$0.0} & 86.0\tiny{$\pm$0.0} & 89.7\tiny{$\pm$0.2} & 89.7\tiny{$\pm$0.1} & 89.6\tiny{$\pm$0.1}\\
       \rowcolor{gray!20}
     \cellcolor{white}  ~ & $\Delta_{\text{NDCG}}$ & 51.6\tiny{$\pm $0.9} & 50.3\tiny{$\pm $1.0} & \textbf{50.1}\tiny{$\pm $1.0}  & 19.1\tiny{$\pm$5.5} & 19.0\tiny{$\pm$5.2} & \textbf{17.9}\tiny{$\pm$6.1} & 38.7\tiny{$\pm$7.2} & 36.0\tiny{$\pm$9.0} & \textbf{34.3}\tiny{$\pm$11.5}\\ % delta ndcg
 \cline{1-11}
       \multirow{3}*{\textbf{GNN-}$\mathbf{S_{0}^{\textbf{Te}}}$} &  $\mathcal{V}^R$ & 85.1\tiny{$\pm $0.7} & 85.3\tiny{$\pm $1.4} & 85.2\tiny{$\pm $1.4} & 85.3\tiny{$\pm$0.6} & 85.4\tiny{$\pm$0.5} & 85.4\tiny{$\pm$0.4} &  89.4\tiny{$\pm$0.6} & 89.6\tiny{$\pm$0.1} & 89.0\tiny{$\pm$0.06} \\
       ~ & $\mathcal{V}^R_1$ & 85.2\tiny{$\pm $0.8} & 83.4\tiny{$\pm $1.3} & 83.5\tiny{$\pm $1.3} & 85.2\tiny{$\pm$0.6} & 85.5\tiny{$\pm$0.4} & 85.5\tiny{$\pm$0.4} & 89.4\tiny{$\pm$0.06} & 89.0\tiny{$\pm$0.01} & 89.1\tiny{$\pm$0.06}\\
       \rowcolor{gray!20}
       \cellcolor{white} ~ & $\Delta_{\text{NDCG}}$ & 51.2\tiny{$\pm $1.5} & 
       \textbf{50.9}\tiny{$\pm $2.4} & \textbf{50.9}\tiny{$\pm $2.3}  & 21.9\tiny{$\pm$6.9}  & 21.9\tiny{$\pm$6.3}  & \textbf{20.9}\tiny{$\pm$9.4} & 38.9\tiny{$\pm$7.6} & 36.9\tiny{$\pm$9.5} & \textbf{34.9}\tiny{$\pm$11.0}\\   % delta ndcg
 \cline{1-11}
        \multirow{3}*{\textbf{GNN-}$\mathbf{S_{1}^{\textbf{Te}}}$} &  $\mathcal{V}^R$ & 84.7\tiny{$\pm $1.3} & 83.7\tiny{$\pm $0.9} & 83.1\tiny{$\pm $0.9}  & 85.7\tiny{$\pm$0.1} & 85.8\tiny{$\pm$0.1} & 85.8\tiny{$\pm$0.2} &  89.6\tiny{$\pm$0.3} & 89.6\tiny{$\pm$0.1} & 89.5\tiny{$\pm$0.3} \\
       ~ & $\mathcal{V}^R_1$ & 84.8\tiny{$\pm $1.3} & 83.9\tiny{$\pm $0.9} & 83.4\tiny{$\pm $0.9} & 85.8\tiny{$\pm$0.1} & 85.8\tiny{$\pm$0.1} & 85.8\tiny{$\pm$0.1} & 89.6\tiny{$\pm$0.3} & 89.6\tiny{$\pm$0.1} & 89.5\tiny{$\pm$0.3}\\
       \rowcolor{gray!20}
       \cellcolor{white} ~ & $\Delta_{\text{NDCG}}$ & 51.3\tiny{$\pm $0.6} & 50.8\tiny{$\pm $0.6} & \textbf{50.2}\tiny{$\pm $1.0}  &  21.0\tiny{$\pm$5.4}  & 19.8\tiny{$\pm$5.4}  & \textbf{19.3}\tiny{$\pm$6.8} & 38.7\tiny{$\pm$7.2} & 36.2\tiny{$\pm$9.5} & \textbf{34.6}\tiny{$\pm$11.4}\\   % delta NDCG
    \bottomrule
    \end{tabular}}
    \label{tab: big table}
    % \vspace{-0.5cm}
\end{table*}
